# Supplementary material for: On the Initialization for Convex-Concave Min-max Problems
Source: arXiv:2103.00284 source file (2022-03-08)
Supplement: Supplementary file 1 [file main_and_appendix.pdf]

# A Parameter-free Algorithm for Convex-Concave Min-max Problems

Anonymous Authors<sup>1</sup>

## Abstract

Parameter-free optimization algorithms refer to algorithms whose convergence rate is optimal with respect to the initial point without any learning rate to tune. They are proposed and well-studied in the online convex optimization literature. However, all the existing parameter-free algorithms can only be used for convex minimization problems. It remains unclear how to design a parameter-free algorithm for convex-concave min-max problems. In fact, the best known convergence rates of the algorithms for solving these problems depend on the size of the domain, rather than on the distance between initial point and the optimal solution. In this paper, we provide the first parameter-free algorithm for several classes of convex-concave problems and establish corresponding state-of-the-art convergence rates, including strictly-convex-strictly-concave min-max problems and min-max problems with non-Euclidean geometry. As a by-product, we utilize the parameter-free algorithm as a subroutine to design a new algorithm, which obtains fast rates for min-max problems with a growth condition. Extensive experiments are conducted to verify our theoretical findings and demonstrate the effectiveness of the proposed algorithm.

## 1. Introduction

In this paper, we are interested in the following problem

$$\min_{\mathbf{x} \in \mathcal{X}} \max_{\mathbf{y} \in \mathcal{Y}} F(\mathbf{x}, \mathbf{y}) \quad (1)$$

where  $\mathcal{X} \subset \mathbb{R}^m$ ,  $\mathcal{Y} \subset \mathbb{R}^n$  are convex and compact sets. This problem has broad applications in machine learning, e.g., stochastic AUC maximization (Ying et al., 2016), generative adversarial nets (Goodfellow et al., 2014), robust

optimization (Ben-Tal et al., 2009), and adversarial training (Madry et al., 2017). In this paper, we consider the case that  $F(\mathbf{x}, \mathbf{y})$  is convex in  $\mathbf{x}$  and concave in  $\mathbf{y}$ .

The canonical method for solving the convex-concave game is the primal-dual gradient method (Nemirovski et al., 2009). For example, in the Euclidean setup, primal-dual gradient method is performing gradient descent on the primal variable  $\mathbf{x}$  and gradient ascent on the dual variable  $\mathbf{y}$  simultaneously. Nemirovski et al. (2009) proved that the averaged solution of primal-dual gradient method has good convergence guarantees in terms of the duality gap, which is

$$\max_{\mathbf{y} \in \mathcal{Y}} F(\bar{\mathbf{x}}_T, \mathbf{y}) - \min_{\mathbf{x} \in \mathcal{X}} F(\mathbf{x}, \bar{\mathbf{y}}_T) \leq \frac{D^2}{2\eta T} + \frac{1}{2}\eta G^2, \quad (2)$$

where  $(\bar{\mathbf{x}}_T, \bar{\mathbf{y}}_T) = (\frac{1}{T} \sum_{t=1}^T \mathbf{x}_t, \frac{1}{T} \sum_{t=1}^T \mathbf{y}_t)$  is the averaged solution,  $D$  is the diameter of the domain,  $G$  is an upper bound on the norm of the gradient. To get the tightest bound for the RHS of (2), we can choose  $\eta = \frac{D}{G\sqrt{T}}$  and end up with  $\frac{DG}{\sqrt{T}}$  bound for the duality gap.

Strangely enough, the optimal learning rate scheme in the primal-dual gradient method completely ignores the effect of the initialization. Regardless of how close the initialization is to the optimal solution, this algorithm ends up with the same complexity guarantees. This is counter-intuitive: we would expect to be able to obtain a faster convergence if the initialization is closer to the optimal solution. Yet, the hardness results in the optimization literature show that  $\Omega(\frac{DG}{\sqrt{T}})$  complexity lower bound is unimprovable (Nemirovskij & Yudin, 1983; Juditsky et al., 2011). This naturally motivates the following question:

*Under mild conditions, can we design a first-order algorithm for solving convex-concave min-max problems, whose computational complexity provably adapts to the distance between initialization and the optimal solution?*

In other words, the goal is to obtain<sup>1</sup>  $\tilde{O}\left(\frac{\text{dist}(\mathbf{x}_0, \mathbf{x}_*) + \text{dist}(\mathbf{y}_0, \mathbf{y}_*)}{\sqrt{T}}\right)$  convergence rate, where  $\text{dist}$  is some metric depending on the geometry of the problem.

We give an affirmative answer to this question by designing a new algorithm called Coin-Betting-Min-Max (CB-Min-

<sup>1</sup>The  $\tilde{O}$  notation hides poly-logarithmic terms.

<sup>1</sup>Anonymous Institution, Anonymous City, Anonymous Region, Anonymous Country. Correspondence to: Anonymous Author <anon.email@domain.com>.

Preliminary work. Under review by the International Conference on Machine Learning (ICML). Do not distribute.

Max). We design our algorithm based on the decoupling of the primal-dual structure and on the coin-betting technique in parameter-free online learning (Orabona & Pál, 2016; Cutkosky & Orabona, 2018a). Specifically, we run a constrained version of coin-betting algorithm on the primal and dual variables simultaneously.

Despite the algorithmic simplicity of our solution, there are two main difficulties in the analysis. First, the definition of the performance metric (e.g., duality gap defined in the LHS of (2)) makes the optimal point achieved in the metric explicitly dependent on the averaged solution of the algorithm, and this particular optimal point may be very different from the optimal solution of the original convex-concave min-max problem. Second, due to the discrepancy between the optimal point achieved in the duality gap and the optimal solution of the original problem, the traditional analysis of parameter-free algorithms does not give initialization-dependent bound with respect to the optimal solution, and hence it can only achieve the worst-case bound which depends on the size of the domain.

To address these issues, we show that the additional assumption of strict convexity/strict concavity of the objective function suffices to prove that our proposed algorithm achieves a convergence rate which explicitly depends on the distance between the initial point and the optimal solution. Several extensions under different settings are also analyzed.

Our contributions are summarized as follows.

- We design a parameter-free algorithm for solving a broad class of convex-concave problems. To the best of our knowledge, this is the first time that a parameter-free algorithm is proposed for min-max problems.
- We prove state-of-the-art convergence rates for the proposed algorithm under various settings, including strictly-convex-strictly-concave min-max problems, and min-max problems with non-euclidean geometry. We also design an algorithm based on the proposed parameter-free algorithm and obtain fast rates for convex-concave min-max problems with a growth condition. To the best our knowledge, leveraging function growth condition to obtain these improved rates for min-max problems is the first shown in this work.
- We verify our theoretical results by conducting both synthetic experiments and distributionally robust optimization on benchmark datasets. We empirically show that our algorithm exhibits good performance in practice.

## 2. Related Work

**Convex-Concave Min-max Optimization** Convex-concave Min-max Optimization is widely studied in

optimization literature, and it is closely related to the variational inequality. The work of (Korpelevich, 1976) proposed the extragradient method for solving variational inequalities, and this was later extended into non-euclidean space (e.g., mirror-prox (Nemirovski, 2004), dual extrapolation (Nesterov, 2007)). The stochastic version of mirror-prox was proposed by (Juditsky et al., 2011). Hsieh et al. (2020) proposed variable stepsize scaling for extragradient method to improve the algorithm’s performance. In nonsmooth case, Nemirovski et al. (2009) analyzed the primal-dual gradient method in non-euclidean space. (Nedić & Ozdaglar, 2009) considered subgradient methods for solving min-max problems and provided per-iteration convergence rate estimates on the solutions. Monteiro & Svaiter (2010) designed hybrid proximal extragradient methods with a different performance measure. Bach & Levy (2019) provided a universal algorithm for solving variational inequalities, which adapts to noise and smoothness.

There are several papers considering specific cases in convex-concave min-max optimization, including functions with a bilinear term (Nesterov, 2005; Chambolle & Pock, 2011; Chen et al., 2014; 2017; He & Monteiro, 2016; Liu et al., 2018; Daskalakis et al., 2018; Liang & Stokes, 2019; Gidel et al., 2019; Mokhtari et al., 2020; Azizian et al., 2020; Bailey et al., 2020), smooth or strongly-convex-(strongly)-concave (Nesterov & Scramali, 2006; Zhao, 2019; Lin et al., 2020; Yan et al., 2020), the last-iterate convergence (Abernethy et al., 2019; Daskalakis & Panageas, 2018; Golowich et al., 2020). There are also some papers about establishing lower bounds in various cases (Ouyang et al., 2013; Zhang et al., 2019; Ibrahim et al., 2020).

However, none of these works provide an upper bound for duality gap which explicitly depends on the distance between the initialization and the optimal solution.

**Parameter-Free Online Convex Optimization** In Online Convex Optimization (OCO) (Gordon, 1999; Zinkevich, 2003), the aim of the learner is to minimize the regret w.r.t. any fixed predictor. Most of the OCO algorithm require some knowledge of the competitor, for example, its norm, in order to achieve the smallest regret (see, e.g., Orabona, 2019). Hence, it becomes impossible to compete *uniformly* with all competitors, unless the algorithm has some knowledge of the future. Morally speaking, the OCO setting is a strict generalization of the setting of stochastic optimization of convex functions and competing with any fixed predictor corresponds exactly to design convex optimization algorithms that have optimal dependency on the distance between the initial point and the optimal solution. Again, without some knowledge of the norm of the optimal solution, classic optimization algorithms fails to get the right dependency.

Parameter-free algorithms avoid setting step sizes completely and get the optimal dependency on the competitor up to poly-log terms (Streeter & McMahan, 2012). The core idea of these algorithms is to use Follow-the-Regularized-Leader<sup>2</sup> (FTRL) (Shalev-Shwartz, 2007; Abernethy et al., 2008) with a time-varying linearithmic (non-strongly convex) regularizer (e.g., Streeter & McMahan, 2012; Orabona, 2014; Cutkosky & Boahen, 2016; 2017; Kotłowski, 2019; Kempka et al., 2019). These algorithms can also be viewed as betting schemes through the duality between regret and reward (McMahan & Orabona, 2014; Orabona & Pál, 2016; Cutkosky & Orabona, 2018a; Cutkosky & Sarlos, 2019).

As far as we know, this is the first application of parameter-free algorithms to convex-concave min-max problems.

### 3. Setting and Assumptions

**Notation** Denote  $\|\cdot\|$  by Euclidean norm. Define  $\langle \cdot, \cdot \rangle$  as the inner product in Euclidean space. Define  $\Pi$  as the orthogonal projection operator. We denote vectors by bold letters, e.g.,  $\mathbf{x}, \mathbf{g}$ .

**Setting and Assumptions** As we said in the introduction, we are interested in the following optimization problem

$$\min_{\mathbf{x} \in \mathcal{X}} \max_{\mathbf{y} \in \mathcal{Y}} F(\mathbf{x}, \mathbf{y}) \quad (3)$$

where  $\mathcal{X} \subset \mathbb{R}^m, \mathcal{Y} \subset \mathbb{R}^n$  are convex and compact sets.

We will assume that  $F$  is convex in the first argument and concave in the second one. Moreover, we assume to have access to a first-order black-box optimization oracle  $\hat{\mathbf{g}} = (\hat{\mathbf{g}}^{\mathbf{x}}, \hat{\mathbf{g}}^{\mathbf{y}})$  at any point  $(\mathbf{x}, \mathbf{y})$ . where  $\hat{\mathbf{g}}^{\mathbf{x}} \in \partial_{\mathbf{x}} F(\mathbf{x}, \mathbf{y})$ , the subgradient of  $F$  w.r.t. its first argument, and  $\hat{\mathbf{g}}^{\mathbf{y}} \in \partial_{\mathbf{y}} (-F(\mathbf{x}, \mathbf{y}))$ , the subgradient of  $-F$  w.r.t. its second argument.

We will also assume that the subgradients  $\hat{\mathbf{g}}^{\mathbf{x}}$  and  $\hat{\mathbf{g}}^{\mathbf{y}}$  have bounded support. In particular, we assume w.l.o.g. that  $\|\hat{\mathbf{g}}^{\mathbf{x}}\| \leq 1$  and  $\|\hat{\mathbf{g}}^{\mathbf{y}}\| \leq 1$  for all  $\mathbf{x} \in \mathcal{X}$  and  $\mathbf{y} \in \mathcal{Y}$ . Note that this assumption is necessary to use parameter-free algorithms (Orabona & Pál, 2016) and it is reasonable because we assume bounded domains.

## 4. Algorithm and Theoretical Analysis

### 4.1. Main Idea

The core idea of our approach is to decouple the primal problem and dual problem in (1), and by then utilize no-regret algorithms to perform the optimization. This is not a new idea by any means, see, for example, (Abernethy et al., 2018). However, we need to be particularly careful

<sup>2</sup>Dual Averaging (Nesterov, 2009) is a specialization of FTRL to linear functions.

### Algorithm 1 Constrained Coin-betting OCO

**Input:** Convex and compact feasible set  $\mathcal{X}$ , initial point  $\mathbf{x}_0 \in \mathcal{X}, \epsilon' > 0$

- 1:  $\tilde{\mathbf{x}}_0 = \mathbf{x}_0$
- 2: **for**  $t = 0, \dots, T - 1$  **do**
- 3:  $\mathbf{x}_t = \Pi_{\mathcal{X}}(\tilde{\mathbf{x}}_t), \mathbf{y}_t = \Pi_{\mathcal{Y}}(\tilde{\mathbf{y}}_t)$
- 4: Receive subgradients  $\hat{\mathbf{g}}_t$
- 5:  $\mathbf{g}_t^{\mathbf{x}} = \frac{1}{2} \left( \hat{\mathbf{g}}_t^{\mathbf{x}} + \|\hat{\mathbf{g}}_t^{\mathbf{x}}\| \cdot \frac{\tilde{\mathbf{x}}_t - \mathbf{x}_t}{\|\tilde{\mathbf{x}}_t - \mathbf{x}_t\|} \right)$  (Define  $\mathbf{0}/\mathbf{0} = \mathbf{0}$ )
- 6:  $\tilde{\mathbf{x}}_{t+1} = -\frac{\sum_{j=1}^t \mathbf{g}_j^{\mathbf{x}}}{t+1} (\epsilon' - \sum_{j=1}^t \langle \mathbf{g}_j^{\mathbf{x}}, \tilde{\mathbf{x}}_j \rangle)$
- 7: **end for**
- 8: **Return**  $\bar{\mathbf{x}}_T = \frac{1}{T} \sum_{t=1}^T \mathbf{x}_t$ .

of the dependency on the initial point. For this reason, we first introduce a Lemma, which is a simple application of Abernethy et al. (2018, Theorem 9).

Suppose to use an OCO algorithm fed with losses  $\ell_t(\mathbf{x}) = F(\mathbf{x}, \mathbf{y}_t)$  that produces the iterates  $\mathbf{x}_t$  and another OCO algorithm fed with losses  $h_t(\mathbf{y}) = -F(\mathbf{x}_t, \mathbf{y})$  that produces the iterates  $\mathbf{y}_t$ . Then, we can state the following Lemma (with detailed proof in Appendix A).

**Lemma 1.** Let  $\bar{\mathbf{x}}_T = \frac{1}{T} \sum_{t=1}^T \mathbf{x}_t, \bar{\mathbf{y}}_T = \frac{1}{T} \sum_{t=1}^T \mathbf{y}_t$ . Then, we have

$$\max_{\mathbf{y} \in \mathcal{Y}} F(\bar{\mathbf{x}}_T, \mathbf{y}) - \min_{\mathbf{x} \in \mathcal{X}} F(\mathbf{x}, \bar{\mathbf{y}}_T) \leq \frac{R_T(\mathbf{x}'_T) + R_T(\mathbf{y}'_T)}{T}, \quad (4)$$

where  $R_T(\mathbf{y}) = \sum_{t=1}^T h_t(\mathbf{y}_t) - \sum_{t=1}^T h_t(\mathbf{y})$ ,  $R_T(\mathbf{x}) = \sum_{t=1}^T \ell_t(\mathbf{x}_t) - \sum_{t=1}^T \ell_t(\mathbf{x})$ ,  $\mathbf{x}'_T \in \arg \min_{\mathbf{x} \in \mathcal{X}} F(\mathbf{x}, \bar{\mathbf{y}}_T)$ , and  $\mathbf{y}'_T \in \arg \max_{\mathbf{y} \in \mathcal{Y}} F(\bar{\mathbf{x}}_T, \mathbf{y})$ .

In words, the above Lemma says that we can use two OCO algorithms to minimize the problem in (2). In particular, the convergence rate depends on the sum of the average regret of the two OCO algorithms. Note that different from similar results, here we care about considering the regret of the OCO algorithms w.r.t. specific points. This will be critical in our improved rates.

### 4.2. Algorithm Design and Analysis

Following the main idea in Section 4.1, our proposed algorithm is presented in Algorithm 2, which can be seen as simultaneous usage of Algorithm 1 on primal variable  $\mathbf{x}$  and dual variable  $\mathbf{y}$ . Algorithm 1 is a parameter-free algorithm which works for constrained problems. The design of Algorithm 1 comes from the unconstrained coin-betting algorithm in (Orabona & Pál, 2016) and a black-box reduction from a constrained coin-betting algorithm to an unconstrained one (Cutkosky & Orabona, 2018b). The idea is to first establish the regret bound of a unconstrained surrogate function  $\tilde{\ell}_t$  over the sequence  $\{\tilde{\mathbf{x}}_t\}$  as in Lemma 2, and then use the black-box reduction to get the regret bound

**Algorithm 2** CB-Min-Max( $\epsilon'$ ,  $\mathbf{x}_0, \mathbf{y}_0, T$ )

**Input:**  $\epsilon' > 0, \mathbf{x}_0 \in \mathcal{X}, \mathbf{y}_0 \in \mathcal{Y}$   
 1:  $\tilde{\mathbf{x}}_0 = \mathbf{x}_0, \tilde{\mathbf{y}}_0 = \mathbf{y}_0$   
 2: **for**  $t = 0, \dots, T-1$  **do**  
 3:    $\mathbf{x}_t = \Pi_{\mathcal{X}}(\tilde{\mathbf{x}}_t), \mathbf{y}_t = \Pi_{\mathcal{Y}}(\tilde{\mathbf{y}}_t)$   
 4:   Receive subgradients  $\hat{\mathbf{g}}_t = (\hat{\mathbf{g}}_t^{\mathbf{x}}, \hat{\mathbf{g}}_t^{\mathbf{y}})$   
 5:    $\mathbf{g}_t^{\mathbf{x}} = \frac{1}{2} \left( \hat{\mathbf{g}}_t^{\mathbf{x}} + \|\hat{\mathbf{g}}_t^{\mathbf{x}}\| \cdot \frac{\tilde{\mathbf{x}}_t - \mathbf{x}_t}{\|\tilde{\mathbf{x}}_t - \mathbf{x}_t\|} \right)$  (Define  $\mathbf{0}/0 = \mathbf{0}$ )  
 6:    $\mathbf{g}_t^{\mathbf{y}} = \frac{1}{2} \left( \hat{\mathbf{g}}_t^{\mathbf{y}} + \|\hat{\mathbf{g}}_t^{\mathbf{y}}\| \cdot \frac{\tilde{\mathbf{y}}_t - \mathbf{y}_t}{\|\tilde{\mathbf{y}}_t - \mathbf{y}_t\|} \right)$  (Define  $\mathbf{0}/0 = \mathbf{0}$ )  
 7:    $\tilde{\mathbf{x}}_{t+1} = -\frac{\sum_{j=1}^t \mathbf{g}_j^{\mathbf{x}}}{t+1} (\epsilon' - \sum_{j=1}^t \langle \mathbf{g}_j^{\mathbf{x}}, \tilde{\mathbf{x}}_j \rangle)$   
 8:    $\tilde{\mathbf{y}}_{t+1} = \frac{\sum_{j=1}^t \mathbf{g}_j^{\mathbf{y}}}{t+1} (\epsilon' + \sum_{j=1}^t \langle \mathbf{g}_j^{\mathbf{y}}, \tilde{\mathbf{y}}_j \rangle)$   
 9: **end for**  
 10: **Return**  $\bar{\mathbf{x}}_T = \frac{1}{T} \sum_{t=1}^T \mathbf{x}_t, \bar{\mathbf{y}}_T = \frac{1}{T} \sum_{t=1}^T \mathbf{y}_t$ .

for the original loss function as in Lemma 3.

Define  $\tilde{\ell}_t(\mathbf{x}) = \frac{1}{2} (\langle \hat{\mathbf{g}}_t^{\mathbf{x}}, \mathbf{x} \rangle + \|\hat{\mathbf{g}}_t^{\mathbf{x}}\| \|\mathbf{x} - \Pi_{\mathcal{X}}(\mathbf{x})\|)$ , then we have the following Lemma.

**Lemma 2.** For  $\forall \mathbf{x} \in \mathcal{X}$ , Algorithm 1 guarantees that

$$\frac{1}{T} \sum_{t=1}^T (\tilde{\ell}_t(\tilde{\mathbf{x}}_t) - \tilde{\ell}_t(\mathbf{x})) \leq O \left( \frac{1}{T} + \frac{\|\mathbf{x}_0 - \mathbf{x}\| \sqrt{\ln(1 + \|\mathbf{x}_0 - \mathbf{x}\|T)}}{\sqrt{T}} \right). \quad (5)$$

*Proof.* Noting that  $\mathbf{g}_t^{\mathbf{x}} \in \partial \tilde{\ell}_t(\tilde{\mathbf{x}}_t)$ , so Algorithm 1 is a coin-betting algorithm for minimizing regret defined by the function  $\tilde{\ell}$  over the sequence of points  $\{\tilde{\mathbf{x}}_t\}$ . Since  $\tilde{\mathbf{x}}_0 = \mathbf{x}_0$ , so by Orabona & Pál (2016, Corollary 5), we immediately get the result.  $\square$

By the black-box reduction illustrated in Cutkosky & Orabona (2018b, Theorem 3) and Lemma 2, we are able to get the following Lemma.

**Lemma 3.** Algorithm 1 guarantees that

$$\begin{aligned} \frac{1}{T} \sum_{t=1}^T \ell_t(\mathbf{x}_t) - \frac{1}{T} \sum_{t=1}^T \ell_t(\mathbf{x}) &\leq 2 \left( \frac{1}{T} \sum_{t=1}^T \tilde{\ell}_t(\tilde{\mathbf{x}}_t) - \frac{1}{T} \sum_{t=1}^T \tilde{\ell}_t(\mathbf{x}) \right) \\ &\leq O \left( \frac{1}{T} + \frac{\|\mathbf{x}_0 - \mathbf{x}\| \sqrt{\ln(1 + \|\mathbf{x}_0 - \mathbf{x}\|T)}}{\sqrt{T}} \right). \end{aligned}$$

Using Lemma 3, Lemma 1, and a parallel argument in terms of the dual variable  $\mathbf{y}$ , we are able to show the following Corollary.

**Corollary 1.** Algorithm 2 guarantees that

$$\begin{aligned} \max_{\mathbf{y} \in \mathcal{Y}} F(\bar{\mathbf{x}}_T, \mathbf{y}) - \min_{\mathbf{x} \in \mathcal{X}} F(\mathbf{x}, \bar{\mathbf{y}}_T) &\leq O \left( \frac{1}{T} + \frac{\|\mathbf{x}_0 - \mathbf{x}'_T\| \sqrt{\ln(1 + \|\mathbf{x}_0 - \mathbf{x}'_T\|T)}}{\sqrt{T}} \right. \\ &\quad \left. + \frac{\|\mathbf{y}_0 - \mathbf{y}'_T\| \sqrt{\ln(1 + \|\mathbf{y}_0 - \mathbf{y}'_T\|T)}}{\sqrt{T}} \right), \end{aligned} \quad (6)$$

where  $\mathbf{x}'_T \in \arg \min_{\mathbf{x} \in \mathcal{X}} F(\mathbf{x}, \bar{\mathbf{y}}_T)$ , and  $\mathbf{y}'_T \in \arg \max_{\mathbf{y} \in \mathcal{Y}} F(\bar{\mathbf{x}}_T, \mathbf{y})$ .

*Proof.* Note that  $h_t(\mathbf{y}) = -F(\mathbf{x}_t, \mathbf{y})$ . A parallel version of Lemma 3 in terms of  $\mathbf{y}$  is

$$\begin{aligned} \frac{1}{T} \sum_{t=1}^T h_t(\mathbf{y}_t) - \frac{1}{T} \sum_{t=1}^T h_t(\mathbf{y}) &\leq O \left( \frac{1}{T} + \frac{\|\mathbf{y}_0 - \mathbf{y}\| \sqrt{\ln(1 + \|\mathbf{y}_0 - \mathbf{y}\|T)}}{\sqrt{T}} \right). \end{aligned} \quad (7)$$

Taking  $\mathbf{x} = \mathbf{x}'_T \in \arg \min_{\mathbf{x} \in \mathcal{X}} F(\mathbf{x}, \bar{\mathbf{y}}_T)$  in Lemma 3,  $\mathbf{y} = \mathbf{y}'_T \in \arg \max_{\mathbf{y} \in \mathcal{Y}} F(\bar{\mathbf{x}}_T, \mathbf{y})$  in (7) and combining Lemma 2, we can prove the Corollary.  $\square$

**Remark:** By Corollary 1, we are able to show that Algorithm 2 enjoys a  $O \left( \frac{D_{\mathcal{X}} \sqrt{\ln(D_{\mathcal{X}}T)} + D_{\mathcal{Y}} \sqrt{\ln(D_{\mathcal{Y}}T)}}{\sqrt{T}} \right)$  convergence rate in terms of duality gap, where  $D_{\mathcal{X}}$  and  $D_{\mathcal{Y}}$  are the diameters of the domain  $\mathcal{X}$  and  $\mathcal{Y}$  respectively. The reason is that we do not know whether  $\mathbf{x}'_T$  ( $\mathbf{y}'_T$ ) is close to  $\mathbf{x}_*$  ( $\mathbf{y}_*$ ) or not, so we cannot get the convergence rate dependent on the distance between the initial point and the optimal solution. In this case, only the worst case bound (dependent on the diameter of the domain) is applicable.

To address this issue, we introduce one mild assumption which helps us obtain the desired bound with explicit dependence on the distance between the initialization and the optimal solution.

In particular, we will use the following assumption:

**Assumption 1.**  $F(\mathbf{x}, \mathbf{y})$  is strictly convex in  $\mathbf{x}$  and strictly concave in  $\mathbf{y}$  and the unique optimal point  $(\mathbf{x}_*, \mathbf{y}_*)$  lies in the interior of  $\mathcal{X} \times \mathcal{Y}$ .

**Remark:** This assumption is crucial to get the desired bound due to the following reasons. First, it can guarantee that both  $\mathbf{x}'_T$  and  $\mathbf{y}'_T$  are unique, which avoid the complicated set-valued analysis. Second, we can utilize this assumption to show that  $\mathbf{x}'_T$  ( $\mathbf{y}'_T$ ) gets close to  $\mathbf{x}_*$  ( $\mathbf{y}_*$ ) when the algorithm runs a sufficiently large number of iterations.

We formalize these insights into the following key Lemma.

**Lemma 4.** Suppose Assumption 1 holds. Define  $\mathbf{x}'_T = \arg \min_{\mathbf{x} \in \mathcal{X}} F(\mathbf{x}, \bar{\mathbf{y}}_T)$ . Then, for Algorithm 2 we have

$$\begin{aligned} & \frac{1}{T} \sum_{t=1}^T \ell_t(\mathbf{x}_t) - \frac{1}{T} \sum_{t=1}^T \ell_t(\mathbf{x}'_T) \\ & \leq O \left( \frac{1}{T} + \frac{\|\mathbf{x}_0 - \mathbf{x}_*\| \sqrt{\ln(1 + \|\mathbf{x}_0 - \mathbf{x}_*\|T)}}{\sqrt{T}} \right). \end{aligned}$$

*Proof.* By Assumption 1, we can uniquely define both  $\mathbf{x}_*$  and  $\mathbf{x}'_T$  as the following:  $\mathbf{x}_* = \arg \min_{\mathbf{x} \in \mathcal{Y}} F(\mathbf{x}, \mathbf{y}_*)$  and  $\mathbf{x}'_T = \arg \min_{\mathbf{x} \in \mathcal{X}} F(\mathbf{x}, \bar{\mathbf{y}}_T)$ .

For brevity of notation, denote by  $C_T(x) = \frac{1}{T} + \frac{x\sqrt{\ln(1+xT)}}{\sqrt{T}}$ . Note that  $C_T(x)$  is non-decreasing in  $x$  and  $\lim_{T \rightarrow \infty} C_T(x) = 0$  for any  $x \in \mathbb{R}_+$ .

Note that

$$\begin{aligned} & \frac{1}{T} \sum_{t=1}^T \ell_t(\mathbf{x}_t) - \frac{1}{T} \sum_{t=1}^T \ell_t(\mathbf{x}'_T) \leq O(C_T(\|\mathbf{x}_0 - \mathbf{x}'_T\|)) \\ & \leq O(C_T(\|\mathbf{x}_0 - \mathbf{x}_*\| + \|\mathbf{x}_* - \mathbf{x}'_T\|)). \end{aligned} \quad (8)$$

By the convergence rate of the Algorithm 2 established in Corollary 1, we know that

$$\begin{aligned} & F(\mathbf{x}_*, \mathbf{y}_*) - F(\mathbf{x}_*, \bar{\mathbf{y}}_T) \leq F(\mathbf{x}_*, \mathbf{y}_*) - \min_{\mathbf{x} \in \mathcal{X}} F(\mathbf{x}, \bar{\mathbf{y}}_T) \\ & \leq \max_{\mathbf{y} \in \mathcal{Y}} F(\bar{\mathbf{x}}_T, \mathbf{y}) - \min_{\mathbf{x} \in \mathcal{X}} F(\mathbf{x}, \bar{\mathbf{y}}_T) \\ & \leq O(C_T(D_{\mathcal{X}}) + C_T(D_{\mathcal{Y}})), \end{aligned} \quad (9)$$

where  $D_{\mathcal{X}}$  is the diameter of  $\mathcal{X}$  and  $D_{\mathcal{Y}}$  is the diameter of  $\mathcal{Y}$ .

We now claim that  $\bar{\mathbf{y}}_T \rightarrow \mathbf{y}_*$  when  $T \rightarrow \infty$ . Let's see why.

Note that  $F(\mathbf{x}, \mathbf{y})$  is strictly concave in terms of  $\mathbf{y}$ . Define  $\tilde{F}(\mathbf{y}) = F(\mathbf{x}_*, \mathbf{y})$ . Taking the limit for  $T \rightarrow \infty$  in (9), for the sequence  $\{\bar{\mathbf{y}}_t\}_{t=1}^\infty$ , we have  $\tilde{F}(\bar{\mathbf{y}}_t) \rightarrow \tilde{F}(\mathbf{y}_*)$ . Given that the domain is bounded, we can extract a convergent subsequence  $\{\bar{\mathbf{y}}_{t_j}\} \subset \{\bar{\mathbf{y}}_t\}$  and we assume that  $\bar{\mathbf{y}}_{t_j} \rightarrow \tilde{\mathbf{y}}$ . By the continuity of  $\tilde{F}(\mathbf{y})$  in terms of  $\mathbf{y}$ , we know that  $\tilde{F}(\bar{\mathbf{y}}_{t_j}) \rightarrow \tilde{F}(\tilde{\mathbf{y}})$ . Now,  $\tilde{F}(\bar{\mathbf{y}}_{t_j})$  is also a subsequence of the convergent sequence  $\tilde{F}(\bar{\mathbf{y}}_t)$ , then  $\tilde{F}(\bar{\mathbf{y}}_{t_j}) \rightarrow \tilde{F}(\mathbf{y}_*)$ . Since  $\mathbf{y}_*$  is uniquely defined, this implies that  $\tilde{\mathbf{y}} = \mathbf{y}_*$ . This means that any convergent subsequence of  $\{\bar{\mathbf{y}}_t\}_{t=1}^\infty$  converges to  $\mathbf{y}_*$ , so  $\bar{\mathbf{y}}_T \rightarrow \mathbf{y}_*$ .

Our next claim is that the mapping  $\arg \min_{\mathbf{x} \in \mathcal{X}} F(\mathbf{x}, \mathbf{y})$  is a continuous function in terms of  $\mathbf{y}$ .

First, define  $H(\mathbf{y}) = \arg \min_{\mathbf{x} \in \mathcal{X}} F(\mathbf{x}, \mathbf{y})$ . By the compactness of  $\mathcal{Y}$ , we have a sequence  $\mathbf{y}_k \rightarrow \mathbf{y}_*$ . Define  $\mathbf{x}_k = H(\mathbf{y}_k)$  and  $\mathbf{x}_* = H(\mathbf{y}_*)$ . By the compactness of  $\mathcal{X}$ , there exists a convergent subsequence  $\mathbf{x}_{k_i}$  of  $\mathbf{x}_k$ ,

and we denote its limit by  $\tilde{\mathbf{x}}$ . From the above, we have  $F(\mathbf{x}_{k_i}, \mathbf{y}_{k_i}) \leq F(\mathbf{x}, \mathbf{y}_{k_i})$  for all  $\mathbf{x} \in \mathcal{X}$ , that implies  $F(\tilde{\mathbf{x}}, \mathbf{y}_*) \leq F(\mathbf{x}, \mathbf{y}_*)$  for any  $\mathbf{x} \in \mathcal{X}$ . In particular, this implies  $F(\tilde{\mathbf{x}}, \mathbf{y}_*) \leq F(\mathbf{x}_*, \mathbf{y}_*)$ . By the uniqueness of the minimizer, we must have  $\tilde{\mathbf{x}} = \mathbf{x}_*$ . Given that any convergent subsequence converges to  $\mathbf{x}_*$ , this means that  $\mathbf{x}_k \rightarrow \mathbf{x}_*$  and hence  $\arg \min_{\mathbf{x} \in \mathcal{X}} F(\mathbf{x}, \mathbf{y})$  is a continuous function in terms of  $\mathbf{y}$ .

Combining the above two claims, by the definition of  $\mathbf{x}_*$  and  $\mathbf{x}'_T$ , we obtain that  $\mathbf{x}'_T \rightarrow \mathbf{x}_*$  when  $T \rightarrow \infty$ . Hence  $\|\mathbf{x}_* - \mathbf{x}'_T\| = o(1)$ . Plugging it in (8), we have

$$\frac{1}{T} \sum_{t=1}^T \ell_t(\mathbf{x}_t) - \frac{1}{T} \sum_{t=1}^T \ell_t(\mathbf{x}'_T) \leq O(C_T(\|\mathbf{x}_0 - \mathbf{x}_*\|)). \quad \square$$

With Lemma 4 and a parallel argument in terms of  $\mathbf{y}$ , we are able to prove the following Theorem 1.

**Theorem 1.** Suppose Assumption 1 holds. Then, Algorithm 2 guarantees that

$$\begin{aligned} & \max_{\mathbf{y} \in \mathcal{Y}} F(\bar{\mathbf{x}}_T, \mathbf{y}) - \min_{\mathbf{x} \in \mathcal{X}} F(\mathbf{x}, \bar{\mathbf{y}}_T) \\ & \leq O \left( \frac{1}{T} + \frac{\|\mathbf{x}_0 - \mathbf{x}_*\| \sqrt{\ln(1 + \|\mathbf{x}_0 - \mathbf{x}_*\|T)}}{\sqrt{T}} \right. \\ & \quad \left. + \frac{\|\mathbf{y}_0 - \mathbf{y}_*\| \sqrt{\ln(1 + \|\mathbf{y}_0 - \mathbf{y}_*\|T)}}{\sqrt{T}} \right). \end{aligned}$$

**Remark:** Theorem 1 shows that Algorithm 2 enjoys a  $\tilde{O}\left(\frac{\text{dist}(\mathbf{x}_0, \mathbf{x}_*) + \text{dist}(\mathbf{y}_0, \mathbf{y}_*)}{\sqrt{T}}\right)$  convergence rate, where  $\text{dist}(\mathbf{a}, \mathbf{b}) = \|\mathbf{a} - \mathbf{b}\|$ .

## 5. Extensions

In this section, we discuss two possible extensions of our Algorithm 2. In Section 5.1, we consider extending our algorithm to the non-Euclidean space. One particular interest is simplex setup, due to emerging applications in distributionally robust optimization (Namkoong & Duchi, 2016). In Section 5.2, we consider an extension of our algorithm when the function satisfies some growth conditions, in which we establish improved rates.

### 5.1. Non-Euclidean Space: Simplex Setup

Min-max optimization in Non-Euclidean spaces is an important topic, which has broad applications in machine learning (e.g., distributionally robust optimization). In this subsection, we focus on the simplex setup by considering the following problem  $\min_{\mathbf{x} \in \mathcal{X}} \max_{\mathbf{p} \in \Delta_n} F(\mathbf{x}, \mathbf{p})$ , where

$$\Delta_n = \left\{ (p_1, p_2, \dots, p_n) \in \mathbb{R}^n \mid 0 \leq p_i \leq 1, \sum_{i=1}^n p_i = 1 \right\}.$$

**Algorithm 3** Simplex-Constrained Coin-betting OCO

**Input:** Simplex  $\Delta_n \in \mathbb{R}^n$ , prior distribution  $\mathbf{p}_0 \in \Delta_n$

- 1: **for**  $t = 1, \dots, T$  **do**
- 2:    $\mathbf{w}_{t,i} = \frac{\sum_{j=1}^{t-1} \tilde{\mathbf{g}}_{j,i}}{t} (1 + \sum_{j=1}^{t-1} \tilde{\mathbf{g}}_{j,i} \mathbf{w}_{j,i}), i = 1, \dots, n$
- 3:    $\hat{\mathbf{p}}_{t,i} = \mathbf{p}_{0,i} \max(\mathbf{w}_{t,i}, 0), i = 1, \dots, n$
- 4:    $\mathbf{p}_t = \hat{\mathbf{p}}_t / \|\hat{\mathbf{p}}_t\|_1$  if  $\|\hat{\mathbf{p}}_t\|_1 \neq 0$  else  $\mathbf{p}_t = \mathbf{p}_0$
- 5:   Receive subgradient  $\mathbf{g}_t^{\mathbf{p}}$
- 6:    $\tilde{\mathbf{g}}_{t,i} = \mathbf{g}_{t,i}^{\mathbf{p}} - \langle \mathbf{g}_t^{\mathbf{p}}, \mathbf{p}_t \rangle$  if  $\mathbf{w}_{t,i} > 0$  else  $\tilde{\mathbf{g}}_{t,i} = \max(\mathbf{g}_{t,i}^{\mathbf{p}} - \langle \mathbf{g}_t^{\mathbf{p}}, \mathbf{p}_t \rangle, 0), i = 1, \dots, n$
- 7: **end for**
- 8: **Return**  $\bar{\mathbf{p}}_T = \frac{1}{T} \sum_{t=1}^T \mathbf{p}_t$

**Algorithm 4** CB-Min-Max-Simplex

**Input:**  $\epsilon', \mathbf{x}_0 \in \mathcal{X}$ , prior distribution  $\mathbf{p}_0 \in \Delta_n$

- 1:  $\tilde{\mathbf{x}}_0 = \mathbf{x}_0$
- 2: **for**  $t = 0, \dots, T$  **do**
- 3:    $\mathbf{x}_t = \Pi_{\mathcal{X}}(\tilde{\mathbf{x}}_t)$
- 4:   Receive Subgradient  $\tilde{\mathbf{g}}_t^{\mathbf{x}}$
- 5:    $\mathbf{g}_t^{\mathbf{x}} = \frac{1}{2} \left( \tilde{\mathbf{g}}_t^{\mathbf{x}} + \|\tilde{\mathbf{g}}_t^{\mathbf{x}}\| \cdot \frac{\tilde{\mathbf{x}}_t - \mathbf{x}_t}{\|\tilde{\mathbf{x}}_t - \mathbf{x}_t\|} \right)$  (Define  $\mathbf{0}/0 = \mathbf{0}$ )
- 6:    $\mathbf{w}_{t,i} = \frac{\sum_{j=1}^{t-1} \tilde{\mathbf{g}}_{j,i}}{t} (1 + \sum_{j=1}^{t-1} \tilde{\mathbf{g}}_{j,i} \mathbf{w}_{j,i}), i = 1, \dots, n$
- 7:    $\hat{\mathbf{p}}_{t,i} = \mathbf{p}_{0,i} \max(\mathbf{w}_{t,i}, 0), i = 1, \dots, n$
- 8:    $\mathbf{p}_t = \hat{\mathbf{p}}_t / \|\hat{\mathbf{p}}_t\|_1$  if  $\|\hat{\mathbf{p}}_t\|_1 \neq 0$  else  $\mathbf{p}_t = \mathbf{p}_0$
- 9:   Receive subgradient  $\tilde{\mathbf{g}}_t^{\mathbf{p}}$
- 10:    $\tilde{\mathbf{g}}_{t,i} = \tilde{\mathbf{g}}_{t,i}^{\mathbf{p}} - \langle \tilde{\mathbf{g}}_t^{\mathbf{p}}, \mathbf{p}_t \rangle$  if  $\mathbf{w}_{t,i} > 0$  else  $\tilde{\mathbf{g}}_{t,i} = \max(\tilde{\mathbf{g}}_{t,i}^{\mathbf{p}} - \langle \tilde{\mathbf{g}}_t^{\mathbf{p}}, \mathbf{p}_t \rangle, 0), i = 1, \dots, n$
- 11:    $\tilde{\mathbf{x}}_{t+1} = -\frac{\sum_{j=1}^t \mathbf{g}_j^{\mathbf{x}}}{t+1} (\epsilon' - \sum_{j=1}^t \langle \mathbf{g}_j^{\mathbf{x}}, \tilde{\mathbf{x}}_j \rangle)$
- 12: **end for**
- 13: **Return**  $\bar{\mathbf{x}}_T = \frac{1}{T} \sum_{t=1}^T \mathbf{x}_t, \bar{\mathbf{p}}_T = \frac{1}{T} \sum_{t=1}^T \mathbf{p}_t$

Our algorithm design shares the similar spirit as in the Euclidean case (Algorithm 2), in which we split the original problem into the primal and dual problems, and employ corresponding coin-betting algorithms for solving them simultaneously. The algorithm is presented in Algorithm 4, which is a synthesis of Algorithm 1 and Algorithm 3. It is worth mentioning that Algorithm 3 is adapted from Algorithm 2 in (Orabona & Pál, 2016), which is a parameter-free coin-betting algorithm in the probability simplex.

The main difficulty of analyzing parameter-free algorithms for min-max problems in a non-Euclidean space is that we have to use a different distance-generating function, and generalize the proofs done in Euclidean space in Section 4 to non-Euclidean spaces.

We first present two key Lemmas (Lemma 5 and Lemma 6) which are useful for our analysis. The proofs are included in Appendix B. Lemma 5 plays the role of the triangle inequality for the KL-divergence, and Lemma 6 provides the non-euclidean variant of (7) in the proof of Corollary 1.

**Lemma 5.** Assume  $\pi$  is a discrete probability distribution

over  $\mathbb{R}^n$  with  $\pi_i > 0$ . Let  $\mathbf{p}, \mathbf{q}$  arbitrary vectors in the probability simplex. Then,

$$KL(\mathbf{p}, \pi) \leq KL(\mathbf{p}, \mathbf{q}) + \max_i \max \left( \ln \frac{q_i}{\pi_i}, 0 \right) \|\mathbf{p} - \mathbf{q}\|_1 + KL(\mathbf{q}, \pi).$$

**Lemma 6.** Define  $h_t(\mathbf{p}) = -F(\mathbf{x}_t, \mathbf{p})$ . Then Algorithm 4 guarantees that for any  $\mathbf{p} \in \Delta_n$ , we have

$$\begin{aligned} & \frac{1}{T} \sum_{t=1}^T h_t(\mathbf{p}_t) - \frac{1}{T} \sum_{t=1}^T h_t(\mathbf{p}) \\ & \leq O \left( \frac{1}{T} + \frac{\sqrt{\ln T + KL(\mathbf{p}, \mathbf{p}_0)}}{\sqrt{T}} \right). \end{aligned} \quad (10)$$

Here we present our main theorem in this section.

**Theorem 2.** Suppose Assumption 1 holds and  $\mathbf{p}_{0,i} > 0$  for every  $i = 1, \dots, n$ . Then Algorithm 4 guarantees that

$$\begin{aligned} & \max_{\mathbf{p} \in \Delta_n} F(\bar{\mathbf{x}}_T, \mathbf{p}) - \min_{\mathbf{x} \in \mathcal{X}} F(\mathbf{x}, \bar{\mathbf{p}}_T) \\ & \leq O \left( \frac{1}{T} + \frac{\|\mathbf{x}_0 - \mathbf{x}_*\| \sqrt{\ln(1 + \|\mathbf{x}_0 - \mathbf{x}_*\| T)}}{\sqrt{T}} \right. \\ & \quad \left. + \frac{\sqrt{\ln T + KL(\mathbf{p}_*, \mathbf{p}_0)}}{\sqrt{T}} \right). \end{aligned}$$

The high-level proof idea of Theorem 2 is to extend the proof of Lemma 4 in Euclidean setting to probability simplex. The main technical ingredient is utilizing the expansion of KL divergence in Lemma 5 and making use of the objective gap bound in Lemma 6. The detailed proof can be found in Appendix B.

## 5.2. Fast Rates: Functions with Growth Condition

In this subsection, we consider the following assumptions.

**Assumption 2.**  $\|\mathbf{x} - \mathbf{x}_*\| \leq c_1 (F(\mathbf{x}, \mathbf{y}_*) - F(\mathbf{x}_*, \mathbf{y}_*))^\theta$  and  $\|\mathbf{y} - \mathbf{y}_*\| \leq c_2 (F(\mathbf{x}_*, \mathbf{y}) - F(\mathbf{x}_*, \mathbf{y}_*))^\theta$ , where  $c_1 > 0$ ,  $c_2 > 0$ ,  $0 < \theta \leq \frac{1}{2}$ ,  $(\mathbf{x}_*, \mathbf{y}_*)$  is the optimal solution of the original problem (1).

**Remark:** The Assumption 2 is a generalization of growth condition in minimization problems (Li, 2013; Yang & Lin, 2018).

**Assumption 3.**  $H_1(\mathbf{y}) = \arg \min_{\mathbf{x} \in \mathcal{X}} F(\mathbf{x}, \mathbf{y})$  is a  $L_{\mathbf{y}}$ -Lipschitz mapping,  $H_2(\mathbf{x}) = \arg \max_{\mathbf{y} \in \mathcal{Y}} F(\mathbf{x}, \mathbf{y})$  is a  $L_{\mathbf{x}}$ -Lipschitz mapping, i.e.,  $\|H_1(\mathbf{y}_1) - H_1(\mathbf{y}_2)\| \leq L_{\mathbf{y}} \|\mathbf{y}_1 - \mathbf{y}_2\|$  for any  $\mathbf{y}_1, \mathbf{y}_2 \in \mathcal{Y}$ , and  $\|H_2(\mathbf{x}_1) - H_2(\mathbf{x}_2)\| \leq L_{\mathbf{x}} \|\mathbf{x}_1 - \mathbf{x}_2\|$  for any  $\mathbf{x}_1, \mathbf{x}_2 \in \mathcal{X}$ .

**Algorithm 5** Restart-CB-Min-Max

**Input:**  $\hat{\mathbf{x}}_0, \hat{\mathbf{y}}_0, \epsilon'$   
 1: **for**  $s = 1, \dots, S$  **do**  
 2:    $(\hat{\mathbf{x}}_s, \hat{\mathbf{y}}_s) = \text{CB-Min-Max}(\epsilon', \hat{\mathbf{x}}_{s-1}, \hat{\mathbf{y}}_{s-1}, T_s)$   
 3: **end for**  
 4: **Return**  $\hat{\mathbf{x}}_S, \hat{\mathbf{y}}_S$

**Remark:** Assumption 3 is closely related to the Aubin Property (Aubin, 1984), which is usually employed to characterize the Lipschitz behavior of solution set for convex optimization problems. Examples satisfying this assumption can be found in (Dontchev & Rockafellar, 2009) (e.g., Example 3B.6, Exercise 3C.5, etc.).

Under Assumption 2 and 3, we can design a restart version of the algorithm, which is presented in Algorithm 5. We will prove that Algorithm 5 enjoys faster convergence rate.

We first provide convergence guarantee for one-stage of Algorithm 5, which is presented in Theorem 3.

**Theorem 3.** Suppose Assumptions 2 and 3 hold. Running 2 for  $T$  iterations yields

$$\begin{aligned} & \max_{\mathbf{y} \in \mathcal{Y}} F(\bar{\mathbf{x}}_T, \mathbf{y}) - \min_{\mathbf{x} \in \mathcal{X}} F(\mathbf{x}, \bar{\mathbf{y}}_T) \\ & \leq O \left( \frac{1}{T} + \frac{1}{T^{\frac{\theta+1}{2}}} + \frac{\text{ObjGap}^\theta(\mathbf{x}_0, \mathbf{y}_0) \ln T}{\sqrt{T}} \right), \end{aligned} \quad (11)$$

where  $\text{ObjGap}(\mathbf{x}_0, \mathbf{y}_0) = [(F(\mathbf{x}_*, \mathbf{y}_0) - F(\mathbf{x}_*, \mathbf{y}_*)) + (F(\mathbf{x}_*, \mathbf{y}_0) - F(\mathbf{x}_*, \mathbf{y}_*))]$ .

*Proof.* Following the proof of Lemma 4, from (8), we know that

$$\begin{aligned} & \frac{1}{T} \sum_{t=1}^T \ell_t(\mathbf{x}_t) - \frac{1}{T} \sum_{t=1}^T \ell_t(\mathbf{x}'_T) \\ & \leq O(C_T(\|\mathbf{x}_0 - \mathbf{x}_*\| + \|\mathbf{x}_* - \mathbf{x}'_T\|)), \end{aligned} \quad (12)$$

where  $\ell_t(\mathbf{x}) = F(\mathbf{x}, \mathbf{y}_t)$ ,  $C_T(x) = \frac{1}{T} + \frac{x\sqrt{\ln(1+Tx)}}{\sqrt{T}}$ ,  $\mathbf{x}'_T = \arg \min_{\mathbf{x}} F(\mathbf{x}, \bar{\mathbf{y}}_T)$ . By the growth condition in Assumption 2, we know that

$$\|\mathbf{x}_0 - \mathbf{x}_*\| \leq c_1 (F(\mathbf{x}_0, \mathbf{y}_*) - F(\mathbf{x}_*, \mathbf{y}_*))^\theta \quad (13)$$

By the Lipschitz property of the argmin map, we have  $\|\mathbf{x}_* - \mathbf{x}'_T\| = \|\arg \min_{\mathbf{x}} F(\mathbf{x}, \mathbf{y}_*) - \arg \min_{\mathbf{x}} F(\mathbf{x}, \bar{\mathbf{y}}_T)\| \leq L_{\mathbf{y}} \|\bar{\mathbf{y}}_T - \mathbf{y}_*\|$ . Note that we have  $\|\bar{\mathbf{y}}_T - \mathbf{y}_*\| \leq c_2 (F(\mathbf{x}_*, \mathbf{y}_*) - F(\mathbf{x}_*, \bar{\mathbf{y}}_T))^\theta$ , so we have

$$\begin{aligned} & \|\mathbf{x}_* - \mathbf{x}'_T\| \leq c_2 L_{\mathbf{y}} (F(\mathbf{x}_*, \mathbf{y}_*) - F(\mathbf{x}_*, \bar{\mathbf{y}}_T))^\theta \\ & \leq c_2 L_{\mathbf{y}} \left( F(\mathbf{x}_*, \mathbf{y}_*) - \min_{\mathbf{x}} F(\mathbf{x}, \bar{\mathbf{y}}_T) \right)^\theta \\ & \leq O \left( \frac{c_2 L_{\mathbf{y}} D_{\mathbf{y}}^\theta \sqrt{\ln(D_{\mathbf{y}} T)}}{T^{\theta/2}} \right), \end{aligned} \quad (14)$$

where the last inequality holds due to the convergence guarantee established in Corollary 1.

Combining (12), (13) and (14), we have

$$\begin{aligned} & \frac{1}{T} \sum_{t=1}^T \ell_t(\mathbf{x}_t) - \frac{1}{T} \sum_{t=1}^T \ell_t(\mathbf{x}'_T) \\ & \leq O \left( \frac{1}{T} + \frac{1}{T^{\frac{\theta+1}{2}}} + \frac{(F(\mathbf{x}_0, \mathbf{y}_*) - F(\mathbf{x}_*, \mathbf{y}_*))^\theta \ln(T)}{\sqrt{T}} \right) \end{aligned} \quad (15)$$

By a parallel argument in terms of  $\mathbf{y}$ , we have

$$\begin{aligned} & \frac{1}{T} \sum_{t=1}^T h_t(\mathbf{y}_t) - \frac{1}{T} \sum_{t=1}^T h_t(\mathbf{y}'_T) \\ & \leq O \left( \frac{1}{T} + \frac{1}{T^{\frac{\theta+1}{2}}} + \frac{(F(\mathbf{x}_*, \mathbf{y}_0) - F(\mathbf{x}_*, \mathbf{y}_*))^\theta \ln(T)}{\sqrt{T}} \right), \end{aligned} \quad (16)$$

where  $h_t(\mathbf{x}) = -F(\mathbf{x}, \mathbf{y}_t)$ ,  $\mathbf{y}'_T = \arg \max_{\mathbf{y}} F(\bar{\mathbf{x}}_T, \mathbf{y})$ . Combining (15) and (16), we know that

$$\begin{aligned} & \max_{\mathbf{y} \in \mathcal{Y}} F(\bar{\mathbf{x}}_T, \mathbf{y}) - \min_{\mathbf{x} \in \mathcal{X}} F(\mathbf{x}, \bar{\mathbf{y}}_T) \\ & \leq O \left( \frac{1}{T} + \frac{1}{T^{\frac{\theta+1}{2}}} + \frac{\text{ObjGap}^\theta(\mathbf{x}_0, \mathbf{y}_0) \ln T}{\sqrt{T}} \right), \end{aligned} \quad (17)$$

where  $\text{ObjGap}(\mathbf{x}_0, \mathbf{y}_0) = [(F(\mathbf{x}_0, \mathbf{y}_*) - F(\mathbf{x}_*, \mathbf{y}_*)) + (F(\mathbf{x}_*, \mathbf{y}_0) - F(\mathbf{x}_*, \mathbf{y}_*))]$ .  $\square$

We then introduce the Theorem 4, which illustrates the improved rate achieved by Algorithm 5.

**Theorem 4.** Suppose Assumptions 2 and 3 hold. Assume  $\text{ObjGap}(\hat{\mathbf{x}}_0, \hat{\mathbf{y}}_0) = [(F(\hat{\mathbf{x}}_0, \mathbf{y}_*) - F(\mathbf{x}_*, \mathbf{y}_*)) + (F(\mathbf{x}_*, \hat{\mathbf{y}}_0) - F(\mathbf{x}_*, \mathbf{y}_*))] \leq \epsilon_0$ . Define  $\epsilon_s = \epsilon_0/2^s$ . Run Algorithm 5 for  $S = \lfloor \log(\epsilon_0/\epsilon) \rfloor$  stages with  $T_s = \tilde{O}(\frac{1}{\epsilon_s^{2-2\theta}})$ , and we can guarantee that  $\max_{\mathbf{y} \in \mathcal{Y}} F(\hat{\mathbf{x}}_S, \mathbf{y}) - \min_{\mathbf{x} \in \mathcal{X}} F(\mathbf{x}, \hat{\mathbf{y}}_S) \leq \epsilon$ . The total iteration complexity is  $\tilde{O}(1/\epsilon^{2(1-\theta)})$ .

*Proof.* Define  $\text{DualityGap}(\hat{\mathbf{x}}_0, \hat{\mathbf{y}}_0) = \max_{\mathbf{y} \in \mathcal{Y}} F(\hat{\mathbf{x}}_0, \mathbf{y}) - \min_{\mathbf{x} \in \mathcal{X}} F(\mathbf{x}, \hat{\mathbf{y}}_0)$ . We know that  $\text{ObjGap}(\hat{\mathbf{x}}_0, \hat{\mathbf{y}}_0) \leq \text{DualityGap}(\hat{\mathbf{x}}_0, \hat{\mathbf{y}}_0)$ . By invoking the subroutine Algorithm 2 to run  $T_0 = \tilde{O}(\frac{1}{\epsilon_0^{2-2\theta}})$  iterations, we know that the duality gap at the new point will be decreased to  $\epsilon_1 = \epsilon_0/2$ . Then the Algorithm 5 restarts by setting the new point as the initial point, and then invokes the subroutine Algorithm 2 to run  $T_1 = \tilde{O}(\frac{1}{\epsilon_1^{2-2\theta}})$  number of iterations, and then it restarts again. Algorithm 5 repeats this process under it reaches  $\epsilon$ -duality gap. We know that we have  $S = \lfloor \log(\epsilon_0/\epsilon) \rfloor$  stages and hence the total complexity is  $\sum_{s=0}^S \tilde{O}(\frac{1}{\epsilon_s^{2-2\theta}}) = \tilde{O}(1/\epsilon^{2(1-\theta)})$ .  $\square$

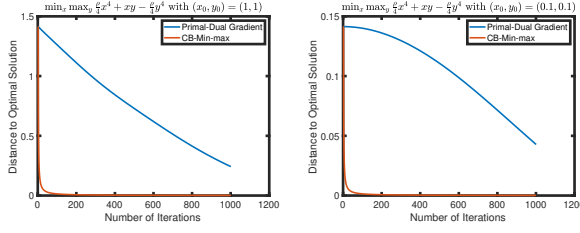

Figure 1. Comparison of different algorithms for the synthetic problem (18) with different initializations (left: starting from (1, 1), right: starting from (0.1, 0.1)). CB-Min-max stands for Algorithm 2.

## 6. Experiments

In this section, we conduct experiments to justify the effectiveness of our proposed algorithm. We consider two problems: one is a synthetic problem, and the another is distributionally robust optimization.

**Synthetic Problem** In the first experiment, we consider the following synthetic min-max problem:

$$\min_{x \in \mathcal{X}} \max_{y \in \mathcal{Y}} F(x, y) := \frac{\rho}{4}x^4 + xy - \frac{\rho}{4}y^4, \quad (18)$$

where  $\mathcal{X} = \{x \mid |x| \leq R_x\}$  and  $\mathcal{Y} = \{y \mid |y| \leq R_y\}$ ,  $\rho, R_x, R_y$  are all positive constants. We can see that the function  $F$  in (18) is an strictly-convex-strictly-concave min-max problem, and the optimal solution is  $(0, 0)$ . In our experiment, we set  $R_x = R_y = 5$ ,  $\rho = 0.5$ . We choose the same initial point  $(x_0, y_0)$  for both primal-dual gradient method with and CB-Min-Max, and report the distance to the optimal solution versus the number of iterations. The learning rate of the primal dual gradient method is set to be  $\frac{D}{G\sqrt{T}}$ , where  $D$  is the diameter of the domain,  $G$  is the gradient's upper bound and  $T$  is the number of iterations. For CB-Min-Max, we set all gradients in Algorithm 2 to be scaled by its upper bound  $G$  to make sure that the scaled gradient has norm smaller than 1. The experimental results are presented in Figure 1. It is observed that for various initialization points, Algorithm 2 consistently converges much faster than the primal-dual gradient method.

**Distributionally Robust Optimization** In the second experiment, we consider the following distributionally robust optimization problem:

$$\min_{\|\mathbf{w}\| \leq R} \max_{\mathbf{p} \in \Delta_n} \sum_{i=1}^n p_i \ell_i(\mathbf{w}) + \frac{\lambda}{2} \left\| \mathbf{p} - \frac{\mathbf{1}_n}{n} \right\|^2 + \frac{\rho}{2} \|\mathbf{w}\|^2, \quad (19)$$

where  $\ell_i(\mathbf{w}) = \max(0, 1 - y_i \mathbf{w}^\top \mathbf{x}_i)$  with  $(\mathbf{x}_i, y_i) \in \mathbb{R}^d \times \{-1, +1\}$  being the feature-label pair and  $\mathbf{w} \in \mathbb{R}^m$  being the model parameter,  $\mathbf{p}$  is a probability vector,  $n$  is the number of training examples,  $\mathbf{1}_n = [1; 1; \dots; 1]$  with length

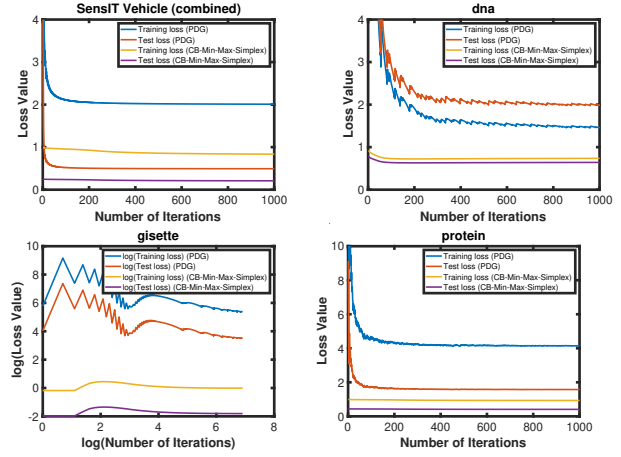

Figure 2. Comparison of different algorithms for the distributionally robust optimization problem (19) on SensIT Vehicle (combined), dna, gisette, protein datasets. PDG stands for primal-dual gradient method, CB-Min-Max-Simplex stands for Algorithm 4.

$n$ . In our experiment, we set  $R = 10^5$ ,  $\lambda = \rho = 10^{-4}$ . Because of the added regularizer, the function becomes strictly-convex-strictly-concave and hence satisfies our Assumption 1. We compare two algorithms: the primal-dual gradient descent (Nemirovski et al., 2009) and our Algorithm 4 (CB-Min-Max-Simplex). In this setup, primal-dual gradient descent method updates  $\mathbf{w}$  by gradient descent and updates  $\mathbf{p}$  by exponential gradient ascent simultaneously. The learning rates are set to be  $\frac{2R}{G_{\mathbf{w}}\sqrt{T}}$  and  $\frac{\log(n)}{G_{\mathbf{p}}\sqrt{T}}$  respectively for primal variable and dual variable, where  $G_{\mathbf{w}}$  is the 2-norm of gradient in terms of  $\mathbf{w}$ , and  $G_{\mathbf{p}}$  is the infinity-norm of the gradient in terms of  $\mathbf{p}$ ,  $T$  is the number of iterations. Both algorithms start from  $\mathbf{w}_0 = 0$ ,  $\mathbf{p}_0 = [1/n; 1/n, \dots, 1/n]$  and run  $T = 1000$  iterations (each iteration amounts to one pass of the training set). We test our algorithms on four benchmark datasets from libsvm website<sup>3</sup> (SensIT Vehicle (combined), dna, gisette, protein). The detailed experimental settings can be found in the Appendix C. We report the training loss and test loss, as shown in the Figure 2. It can be observed that our proposed parameter-free algorithm (i.e., Algorithm 4) significantly outperforms the standard primal-dual gradient method.

## 7. Conclusion

In this paper, we design and analyze the first parameter-free algorithm for a class of convex-concave min-max problems. Various extensions are proposed, including min-max problems with non-Euclidean geometry and fast rate results for min-max problems with function growth condition. Experimental results show the superior performance of the proposed algorithm. In the future, we plan to study the lower bound for parameter-free algorithms in min-max problems.

<sup>3</sup><https://www.csie.ntu.edu.tw/~cjlin/libsvmtools/datasets/>

## References

- Abernethy, J., Lai, K. A., Levy, K. Y., and Wang, J.-K. Faster rates for convex-concave games. *arXiv preprint arXiv:1805.06792*, 2018.
- Abernethy, J., Lai, K. A., and Wibisono, A. Last-iterate convergence rates for min-max optimization. *arXiv preprint arXiv:1906.02027*, 2019.
- Abernethy, J. D., Hazan, E., and Rakhlin, A. Competing in the dark: An efficient algorithm for bandit linear optimization. In Servedio, R. A. and Zhang, T. (eds.), *Proc. of Conference on Learning Theory (COLT)*, pp. 263–274. Omnipress, 2008.
- Aubin, J.-P. Lipschitz behavior of solutions to convex minimization problems. *Mathematics of Operations Research*, 9(1):87–111, 1984.
- Azizian, W., Scieur, D., Mitliagkas, I., Lacoste-Julien, S., and Gidel, G. Accelerating smooth games by manipulating spectral shapes. In *International Conference on Artificial Intelligence and Statistics*, pp. 1705–1715. PMLR, 2020.
- Bach, F. and Levy, K. Y. A universal algorithm for variational inequalities adaptive to smoothness and noise. In *Conference on Learning Theory*, pp. 164–194. PMLR, 2019.
- Bailey, J. P., Gidel, G., and Piliouras, G. Finite regret and cycles with fixed step-size via alternating gradient descent-ascent. In *Conference on Learning Theory*, pp. 391–407. PMLR, 2020.
- Ben-Tal, A., El Ghaoui, L., and Nemirovski, A. *Robust optimization*. Princeton university press, 2009.
- Chambolle, A. and Pock, T. A first-order primal-dual algorithm for convex problems with applications to imaging. *Journal of mathematical imaging and vision*, 40(1):120–145, 2011.
- Chen, Y., Lan, G., and Ouyang, Y. Optimal primal-dual methods for a class of saddle point problems. *SIAM Journal on Optimization*, 24(4):1779–1814, 2014.
- Chen, Y., Lan, G., and Ouyang, Y. Accelerated schemes for a class of variational inequalities. *Mathematical Programming*, 165(1):113–149, 2017.
- Cutkosky, A. and Boahen, K. Online learning without prior information. In *Proc. of the 2017 Conference on Learning Theory*, volume 65 of *Proc. of Machine Learning Research*, pp. 643–677, Amsterdam, Netherlands, 07–10 Jul 2017. PMLR.
- Cutkosky, A. and Boahen, K. A. Online convex optimization with unconstrained domains and losses. In *Advances in Neural Information Processing Systems*, pp. 748–756, 2016.
- Cutkosky, A. and Orabona, F. Black-box reductions for parameter-free online learning in Banach spaces. In *Proc. of the Conference on Learning Theory (COLT)*, 2018a.
- Cutkosky, A. and Orabona, F. Black-box reductions for parameter-free online learning in Banach spaces. *arXiv preprint arXiv:1802.06293*, 2018b.
- Cutkosky, A. and Sarlos, T. Matrix-free preconditioning in online learning. In *International Conference on Machine Learning*, pp. 1455–1464. PMLR, 2019.
- Daskalakis, C. and Panageas, I. Last-iterate convergence: Zero-sum games and constrained min-max optimization. *arXiv preprint arXiv:1807.04252*, 2018.
- Daskalakis, C., Ilyas, A., Syrgkanis, V., and Zeng, H. Training GANs with optimism. In *International Conference on Learning Representations*, 2018.
- Dontchev, A. L. and Rockafellar, R. T. *Implicit functions and solution mappings*, volume 543. Springer, 2009.
- Gidel, G., Hemmat, R. A., Pezeshki, M., Le Priol, R., Huang, G., Lacoste-Julien, S., and Mitliagkas, I. Negative momentum for improved game dynamics. In *The 22nd International Conference on Artificial Intelligence and Statistics*, pp. 1802–1811. PMLR, 2019.
- Golowich, N., Pattathil, S., Daskalakis, C., and Ozdaglar, A. Last iterate is slower than averaged iterate in smooth convex-concave saddle point problems. In *Conference on Learning Theory*, pp. 1758–1784. PMLR, 2020.
- Goodfellow, I., Pouget-Abadie, J., Mirza, M., Xu, B., Warde-Farley, D., Ozair, S., Courville, A., and Bengio, Y. Generative adversarial nets. In *Advances in neural information processing systems*, pp. 2672–2680, 2014.
- Gordon, G. J. Regret bounds for prediction problems. In *Proc. of the twelfth annual conference on Computational learning theory (COLT)*, pp. 29–40, 1999.
- He, Y. and Monteiro, R. D. An accelerated hpe-type algorithm for a class of composite convex-concave saddle-point problems. *SIAM Journal on Optimization*, 26(1): 29–56, 2016.
- Hsieh, Y.-G., Iutzeler, F., Malick, J., and Mertikopoulos, P. Explore aggressively, update conservatively: Stochastic extragradient methods with variable stepsize scaling. *arXiv preprint arXiv:2003.10162*, 2020.

- Ibrahim, A., Azizian, W., Gidel, G., and Mitliagkas, I. Linear lower bounds and conditioning of differentiable games. In *International Conference on Machine Learning*, pp. 4583–4593. PMLR, 2020.
- Juditsky, A., Nemirovski, A., Tauvel, C., et al. Solving variational inequalities with stochastic mirror-prox algorithm. *Stochastic Systems*, 1(1):17–58, 2011.
- Kempka, M., Kotłowski, W., and Warmuth, M. K. Adaptive scale-invariant online algorithms for learning linear models. In Chaudhuri, K. and Salakhutdinov, R. (eds.), *Proc. of the 36th International Conference on Machine Learning*, volume 97 of *Proc. of Machine Learning Research*, pp. 3321–3330, Long Beach, California, USA, 09–15 Jun 2019. PMLR.
- Korpelevich, G. The extragradient method for finding saddle points and other problems. *Matecon*, 12:747–756, 1976.
- Kotłowski, W. Scale-invariant unconstrained online learning. *Theoretical Computer Science*, 2019.
- Li, G. Global error bounds for piecewise convex polynomials. *Mathematical Programming*, pp. 1–28, 2013.
- Liang, T. and Stokes, J. Interaction matters: A note on non-asymptotic local convergence of generative adversarial networks. In *The 22nd International Conference on Artificial Intelligence and Statistics*, pp. 907–915. PMLR, 2019.
- Lin, T., Jin, C., and Jordan, M. I. Near-optimal algorithms for minimax optimization. In *Conference on Learning Theory*, pp. 2738–2779. PMLR, 2020.
- Liu, M., Zhang, X., Chen, Z., Wang, X., and Yang, T. Fast stochastic auc maximization with  $o(1/n)$ -onvergence rate. In *International Conference on Machine Learning*, pp. 3195–3203, 2018.
- Madry, A., Makelov, A., Schmidt, L., Tsipras, D., and Vladu, A. Towards deep learning models resistant to adversarial attacks. *arXiv preprint arXiv:1706.06083*, 2017.
- McMahan, H. B. and Orabona, F. Unconstrained online linear learning in Hilbert spaces: Minimax algorithms and normal approximations. In *Proc of the Annual Conference on Learning Theory, COLT*, 2014.
- Mokhtari, A., Ozdaglar, A., and Pattathil, S. A unified analysis of extra-gradient and optimistic gradient methods for saddle point problems: Proximal point approach. In *International Conference on Artificial Intelligence and Statistics*, pp. 1497–1507. PMLR, 2020.
- Monteiro, R. D. and Svaiter, B. F. On the complexity of the hybrid proximal extragradient method for the iterates and the ergodic mean. *SIAM Journal on Optimization*, 20(6): 2755–2787, 2010.
- Namkoong, H. and Duchi, J. C. Stochastic gradient methods for distributionally robust optimization with f-divergences. In *NIPS*, volume 29, pp. 2208–2216, 2016.
- Nedić, A. and Ozdaglar, A. Subgradient methods for saddle-point problems. *Journal of optimization theory and applications*, 142(1):205–228, 2009.
- Nemirovski, A. Prox-method with rate of convergence  $o(1/t)$  for variational inequalities with lipschitz continuous monotone operators and smooth convex-concave saddle point problems. *SIAM Journal on Optimization*, 15(1): 229–251, 2004.
- Nemirovski, A., Juditsky, A., Lan, G., and Shapiro, A. Robust stochastic approximation approach to stochastic programming. *SIAM Journal on optimization*, 19(4):1574–1609, 2009.
- Nemirovskij, A. S. and Yudin, D. B. Problem complexity and method efficiency in optimization. 1983.
- Nesterov, Y. Smooth minimization of non-smooth functions. *Mathematical programming*, 103(1):127–152, 2005.
- Nesterov, Y. Dual extrapolation and its applications to solving variational inequalities and related problems. *Mathematical Programming*, 109(2):319–344, 2007.
- Nesterov, Y. Primal-dual subgradient methods for convex problems. *Mathematical programming*, 120(1):221–259, 2009.
- Nesterov, Y. and Scramali, L. Solving strongly monotone variational and quasi-variational inequalities. *Available at SSRN 970903*, 2006.
- Orabona, F. Simultaneous model selection and optimization through parameter-free stochastic learning. In *Advances in Neural Information Processing Systems 27*, 2014.
- Orabona, F. A modern introduction to online learning. *arXiv preprint arXiv:1912.13213*, 2019.
- Orabona, F. and Pál, D. Coin betting and parameter-free online learning. In Lee, D. D., Sugiyama, M., Luxburg, U. V., Guyon, I., and Garnett, R. (eds.), *Advances in Neural Information Processing Systems 29*, pp. 577–585. Curran Associates, Inc., 2016.
- Orabona, F. and Pál, D. Coin betting and parameter-free online learning. *arXiv preprint arXiv:1602.04128*, 2016.

- Ouyang, H., He, N., Tran, L., and Gray, A. G. Stochastic alternating direction method of multipliers. *ICML (1)*, 28: 80–88, 2013.
- Shalev-Shwartz, S. *Online Learning: Theory, Algorithms, and Applications*. PhD thesis, The Hebrew University, 2007.
- Streeter, M. and McMahan, B. No-regret algorithms for unconstrained online convex optimization. In *Advances in Neural Information Processing Systems 25*, pp. 2402–2410. Curran Associates, Inc., 2012.
- Yan, Y., Xu, Y., Lin, Q., Liu, W., and Yang, T. Optimal epoch stochastic gradient descent ascent methods for min-max optimization. *Advances in Neural Information Processing Systems*, 33, 2020.
- Yang, T. and Lin, Q. Rsg: Beating subgradient method without smoothness and strong convexity. *The Journal of Machine Learning Research*, 19(1):236–268, 2018.
- Ying, Y., Wen, L., and Lyu, S. Stochastic online auc maximization. In *Advances in Neural Information Processing Systems*, pp. 451–459, 2016.
- Zhang, J., Hong, M., and Zhang, S. On lower iteration complexity bounds for the saddle point problems. *arXiv preprint arXiv:1912.07481*, 2019.
- Zhao, R. Optimal stochastic algorithms for convex-concave saddle-point problems. *arXiv preprint arXiv:1903.01687*, 2019.
- Zinkevich, M. Online convex programming and generalized infinitesimal gradient ascent. In *Proc. of ICML*, pp. 928–936, 2003.

## A. Proofs in Section 4

### A.1. Proof of Lemma 1

*Proof.* Note that  $\ell_t(\mathbf{x}) = F(\mathbf{x}, \mathbf{y}_t)$ , and  $h_t(\mathbf{y}) = -F(\mathbf{x}_t, \mathbf{y})$ . By Jensen's inequality, we have

$$\begin{aligned} F(\bar{\mathbf{x}}_T, \mathbf{y}) - F(\mathbf{x}, \bar{\mathbf{y}}_T) &\leq \frac{1}{T} \sum_{t=1}^T F(\mathbf{x}_t, \mathbf{y}) - \frac{1}{T} \sum_{t=1}^T F(\mathbf{x}, \mathbf{y}_t) \\ &= \frac{1}{T} \sum_{t=1}^T F(\mathbf{x}_t, \mathbf{y}) - \frac{1}{T} \sum_{t=1}^T F(\mathbf{x}_t, \mathbf{y}_t) \\ &\quad + \frac{1}{T} \sum_{t=1}^T F(\mathbf{x}_t, \mathbf{y}_t) - \frac{1}{T} \sum_{t=1}^T F(\mathbf{x}, \mathbf{y}_t) \\ &= \frac{1}{T} \sum_{t=1}^T (h_t(\mathbf{y}_t) - h_t(\mathbf{y})) + \frac{1}{T} \sum_{t=1}^T (\ell_t(\mathbf{x}_t) - \ell_t(\mathbf{x})). \end{aligned}$$

Taking  $\mathbf{x} = \mathbf{x}'_T \in \arg \min_{\mathbf{x} \in \mathcal{X}} F(\mathbf{x}, \bar{\mathbf{y}}_T)$  and  $\mathbf{y} = \mathbf{y}'_T \in \arg \max_{\mathbf{y} \in \mathcal{Y}} F(\bar{\mathbf{x}}_T, \mathbf{y})$ , we get the stated result.  $\square$

## B. Proofs in Section 5.1

### B.1. Proof of Lemma 5

*Proof.*

$$\begin{aligned} KL(\mathbf{p}, \boldsymbol{\pi}) &= \sum_{i=1}^d p_i \ln \frac{p_i}{\pi_i} = \sum_{i=1}^d p_i \ln \frac{p_i}{q_i} + \sum_{i=1}^d p_i \ln \frac{q_i}{\pi_i} \\ &= KL(\mathbf{q}, \boldsymbol{\pi}) + \sum_{i=1}^d q_i \ln \frac{q_i}{\pi_i} + \sum_{i=1}^d (p_i - q_i) \ln \frac{q_i}{\pi_i} \\ &\leq KL(\mathbf{q}, \boldsymbol{\pi}) + \sum_{i=1}^d q_i \ln \frac{q_i}{\pi_i} + \max_i \max(\ln \frac{q_i}{\pi_i}, 0) \sum_{i=1}^d |p_i - q_i|. \end{aligned}$$

### B.2. Proof of Lemma 6

*Proof.* The proof follows Corollary 6 in (Orabona & Pál, 2016) and Jensen's inequality in terms of  $\mathbf{p}$ .  $\square$

### B.3. Proof of Theorem 2

*Proof.* By combining Lemma 6, Lemma 2 and Lemma 1, we can get the following bound

$$\begin{aligned} &\max_{\mathbf{p} \in \Delta_n} F(\bar{\mathbf{x}}_T, \mathbf{p}) - \min_{\mathbf{x} \in \mathcal{X}} F(\mathbf{x}, \bar{\mathbf{p}}_T) \\ &\leq O \left( \frac{1}{T} + \frac{\|\mathbf{x}_0 - \mathbf{x}'_T\| \sqrt{\ln(1 + \|\mathbf{x}_0 - \mathbf{x}_*\|T)}}{\sqrt{T}} \right. \\ &\quad \left. + \frac{\sqrt{\ln T + KL(\mathbf{p}'_T, \mathbf{p}_0)}}{\sqrt{T}} \right), \end{aligned} \tag{20}$$

where  $\mathbf{x}'_T = \arg \min_{\mathbf{x} \in \mathcal{X}} F(\mathbf{x}, \bar{\mathbf{p}}_T)$  and  $\mathbf{p}'_T = \arg \max_{\mathbf{p} \in \Delta_n} F(\bar{\mathbf{x}}_T, \mathbf{p})$ . Note that (20) is the counterpart of Corollary 1 in the probability simplex setup. By Lemma 6 (taking  $\boldsymbol{\pi} = \mathbf{p}_0$ ,  $\mathbf{p} = \mathbf{p}'_T$  and  $\mathbf{q} = \mathbf{p}_*$ ), we know that

$$\begin{aligned} KL(\mathbf{p}'_T, \mathbf{p}_0) &\leq KL(\mathbf{p}'_T, \mathbf{p}_*) \\ &\quad + \max_i \max \left( \ln \frac{\mathbf{p}_{*,i}}{\mathbf{p}_{0,i}}, 0 \right) \|\mathbf{p}'_T - \mathbf{p}_*\|_1 + KL(\mathbf{p}_*, \mathbf{p}_0). \end{aligned} \tag{21}$$

Then, we are able to follow the proof of Lemma 4 to show that  $KL(\mathbf{p}'_T, \mathbf{p}_*) \rightarrow 0$  (this implies that  $\max_i \max \left( \ln \frac{\mathbf{p}_{*,i}}{\mathbf{p}_{0,i}}, 0 \right) \|\mathbf{p}'_T - \mathbf{p}_*\|_1 \rightarrow 0$  by Pinsker's inequality). In addition, it is proved in Lemma 4 that  $\mathbf{x}'_T \rightarrow \mathbf{x}_*$ . Combining these facts with (21), the theorem is proved.  $\square$

### C. Detailed Experimental Settings

- SensIT Vehicle (combined): all the classes with label 2 and 3 are regarded as class  $-1$ , and the class 1 is regarded as class 1.
- dna: all the classes with label 2 and 3 are regarded as class  $-1$ , and the class 1 is regarded as class 1.
- gisette: we use the original dataset without any preprocessing.
- protein: all the classes with label 0 and 2 are regarded as class  $-1$ , and the class 1 is regarded as class 1.
